# Supplementary material for: LinearSankoff: Linear-time Simultaneous Folding and Alignment of RNA Homologs
Source: arXiv:2307.09580 source file (2023-07-18)
Supplement: Supplementary file 1 [file si.tex]

% !TEX root = main.tex

%\section{Section title of first appendix}\label{sec11}
%XXX
%\subsection{Subsection title of first appendix}\label{subsec4}
%XXX
%\subsubsection{Subsubsection title of first appendix}\label{subsubsec3}
%XXX

\begin{figure}[t]
\center
\includegraphics[width=1\linewidth, trim={230 260 230 260}, clip]{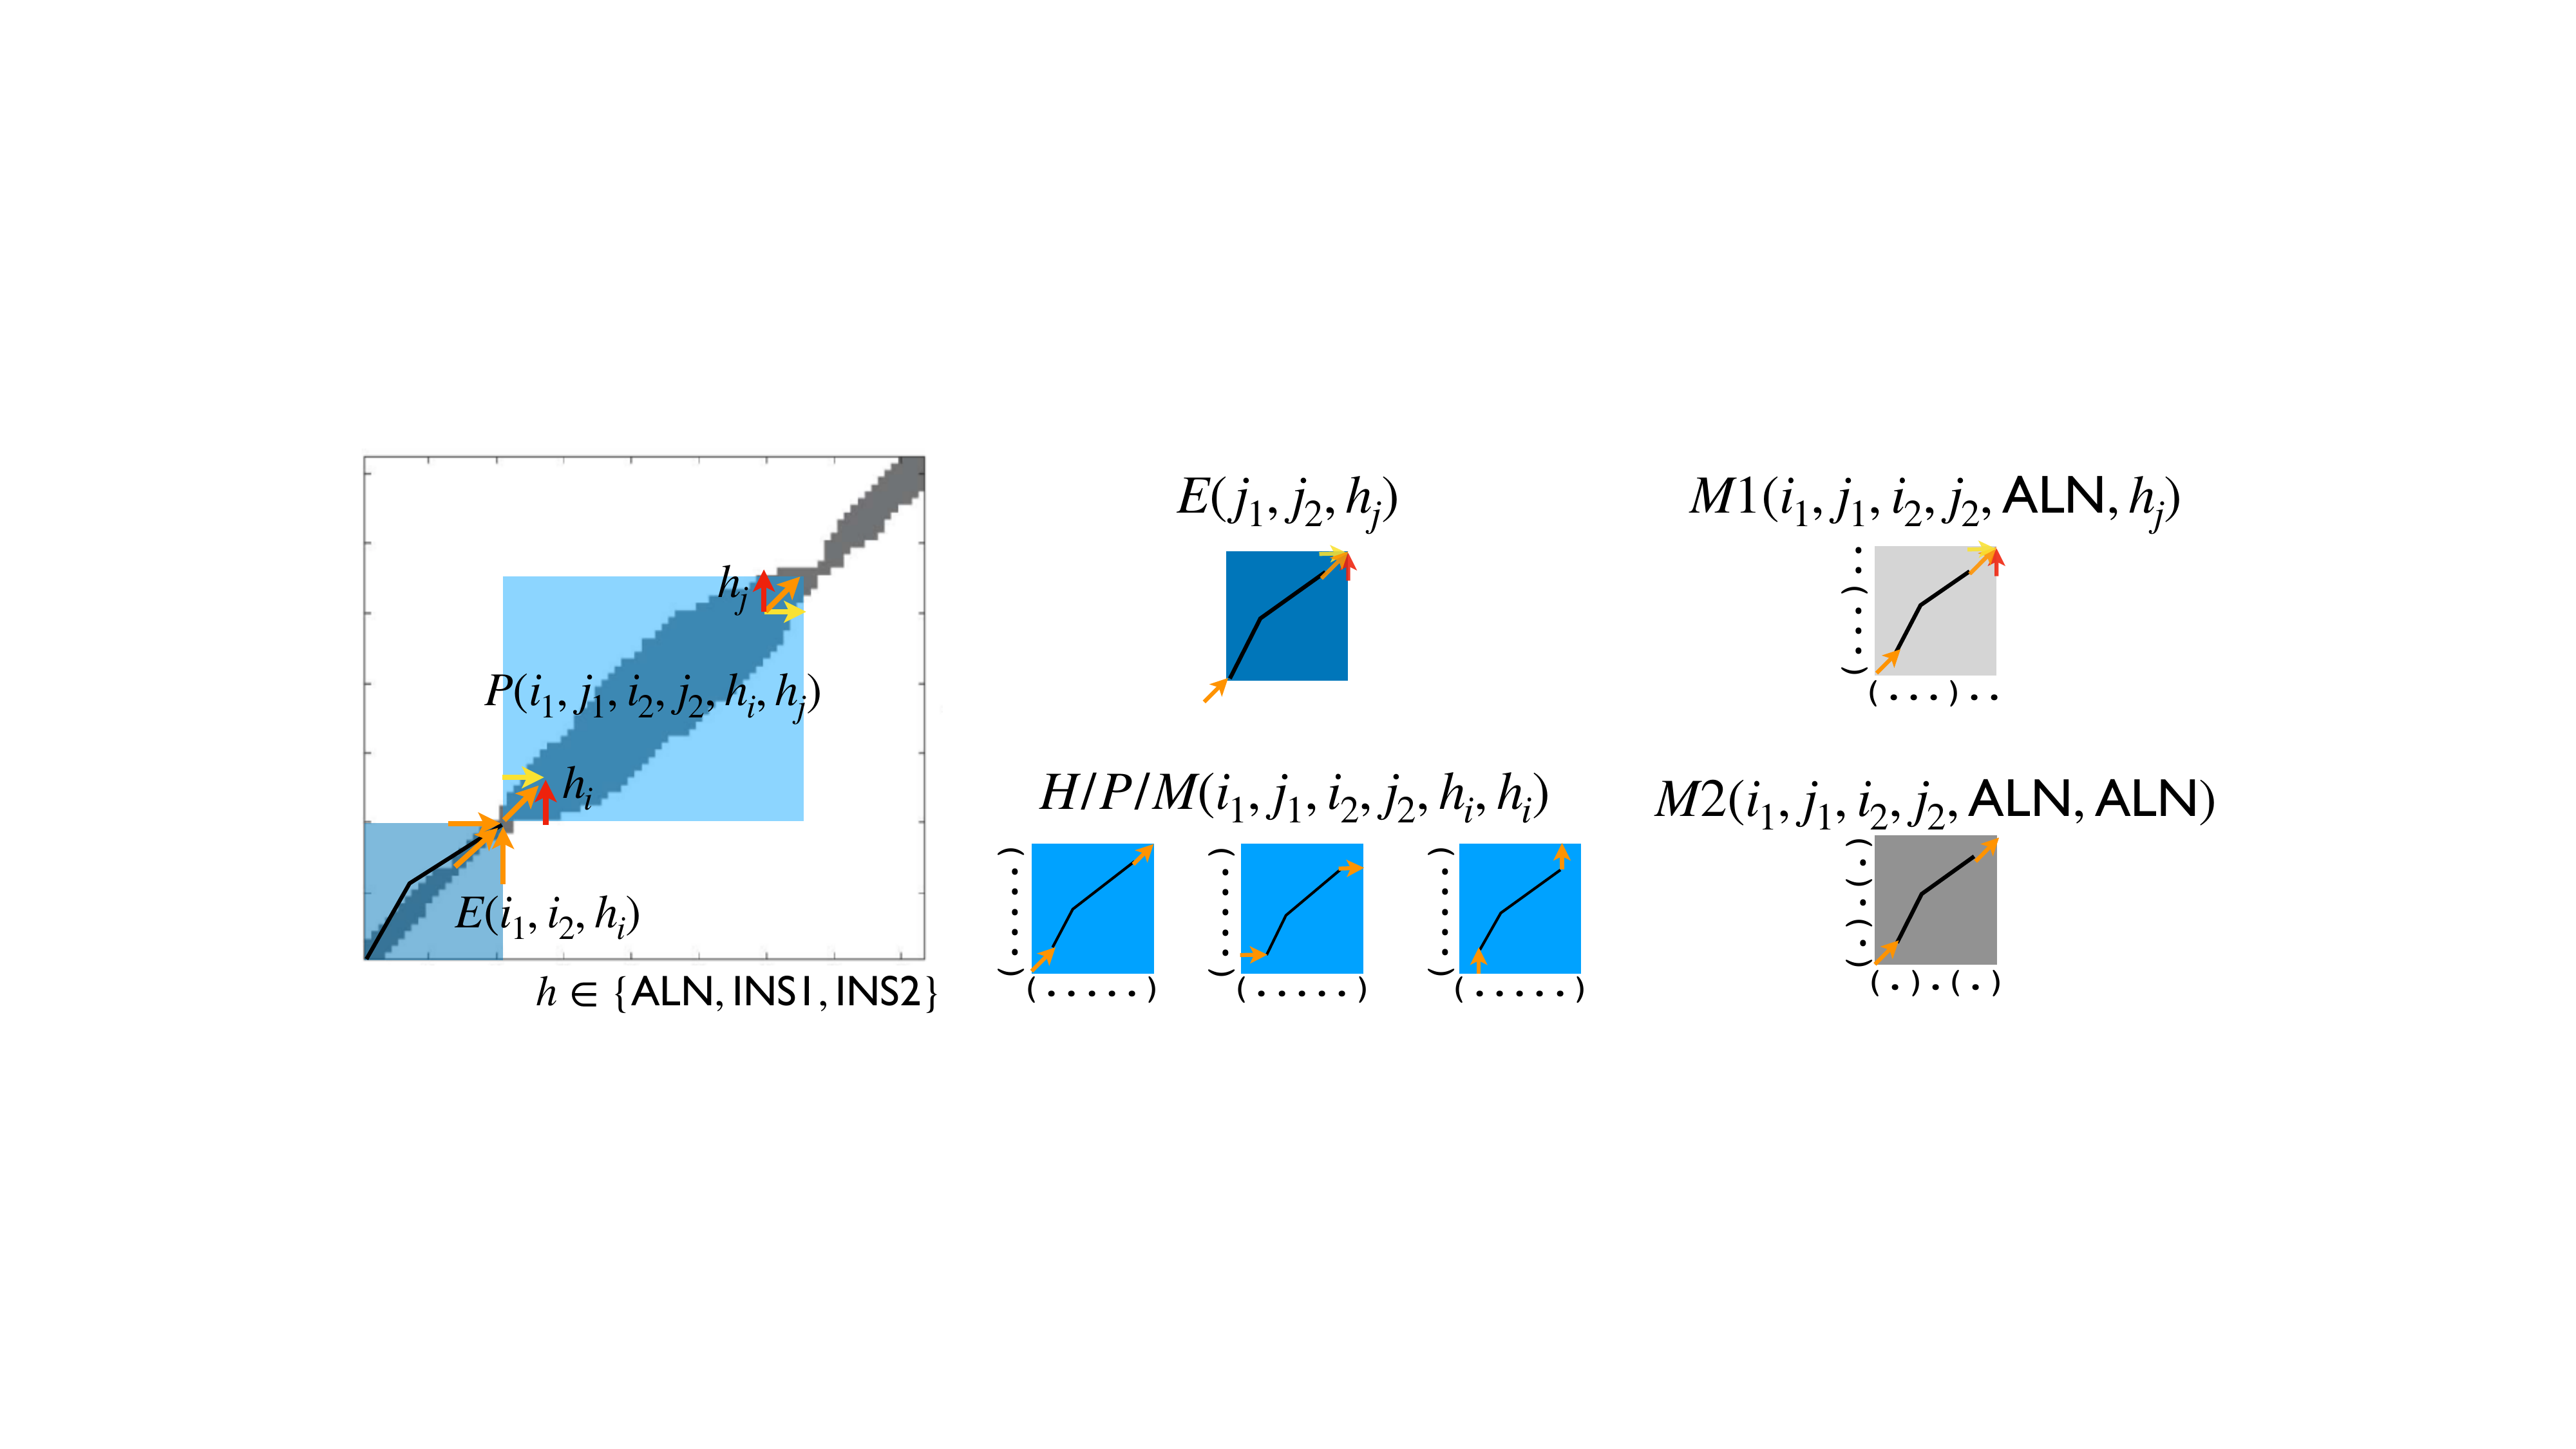} 
%\hfill
\caption[LinearSankoff States]{Examples of \lso states.
The black curves in the rectangles represent the Viterbi alignment path with arrays on the two ends showing different alignment states. 
Dot-bracket structures are annotated along x- and y- axes to indicate different types of structural components. 
% The partition function computation takes about half of the total time shown here.
\label{fig:lso_states}}
\end{figure}
